# Supplementary material for: Automation is no barrier to light vehicle electrification
Source: arXiv:1908.08920 source file (2020-02-06)
Supplement: Supplementary file 1 [file SI.pdf]

# Supporting Information:
# Automation is no barrier to light vehicle electrification


Aniruddh Mohan[1], Shashank Sripad[2], Parth Vaishnav[1,3] & Venkatasubramanian Viswanathan[2,3]

[1]*Department of Engineering and Public Policy, Carnegie Mellon University, Pittsburgh, Pennsylvania, 15213, USA.*

[2]*Department of Mechanical Engineering, Carnegie Mellon University, Pittsburgh, Pennsylvania, 15213, USA.*

[3]*Wilton E. Scott Institute for Energy Innovation, Carnegie Mellon University, Pittsburgh,Pennsylvania, 15213, USA.*

## Contents


1 Drive Profiles 3

2 Smoothing of Composite Drive Profile 4

3 Smoothing of City Drive Profile 5

4 Box Plot results for different EV models (city profile) 8

5 Sensitivity analysis of results 10

6 Battery degradation results 11

7 Costs of automation: Willingness to pay 14

# 1 Drive Profiles

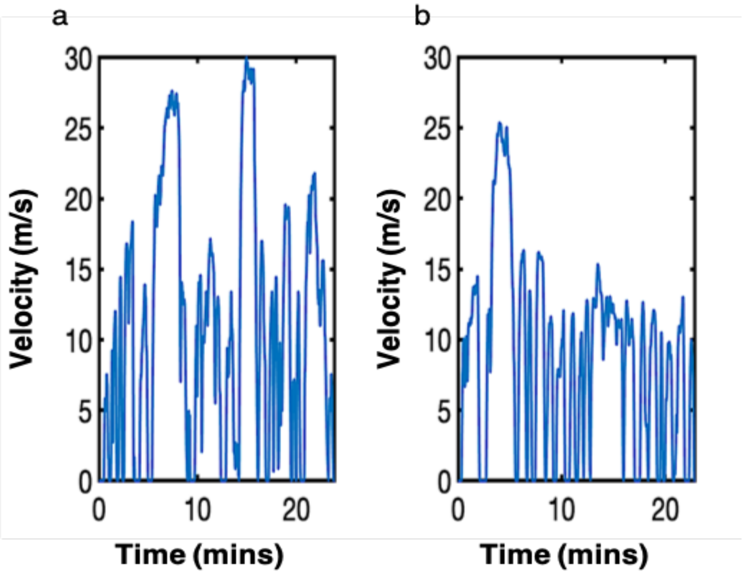


**Figure S1:** **a**, Drive profile for the composite cycle as per the California Unified Cycle Driving Schedule. The maximum speed reached is 67.2 mph. The average driving speed is 29.4 mph. The vehicle comes to rest 16 times during the drive. **b**, Drive profile for the city cycle as per the Urban Dynamometer Driving Schedule. The maximum speed reached is 56.7 mph and the average driving speed is 24.1 mph. The vehicle comes to rest 17 times during the drive.

## 2 Smoothing of Composite Drive Profile

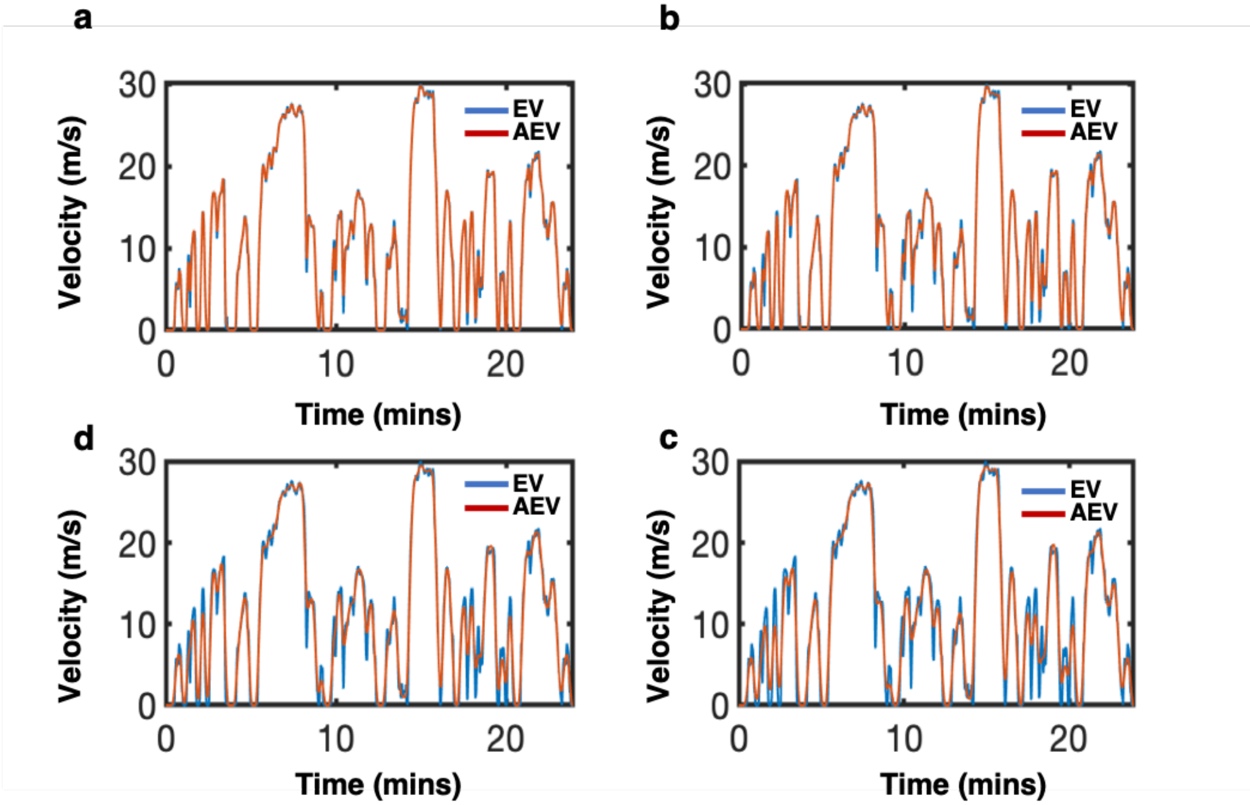


**Figure S2:** Composite Cycle: Clockwise from left to right **a**, AEV vs EV drive cycle for 5% energy savings, **b**, AEV vs V drive cycle for 10% energy savings. **c**, AEV vs EV drive cycle for 20% energy savings. **d**, AEV vs EV drive cycle for 25% energy savings

## 3 Smoothing of City Drive Profile

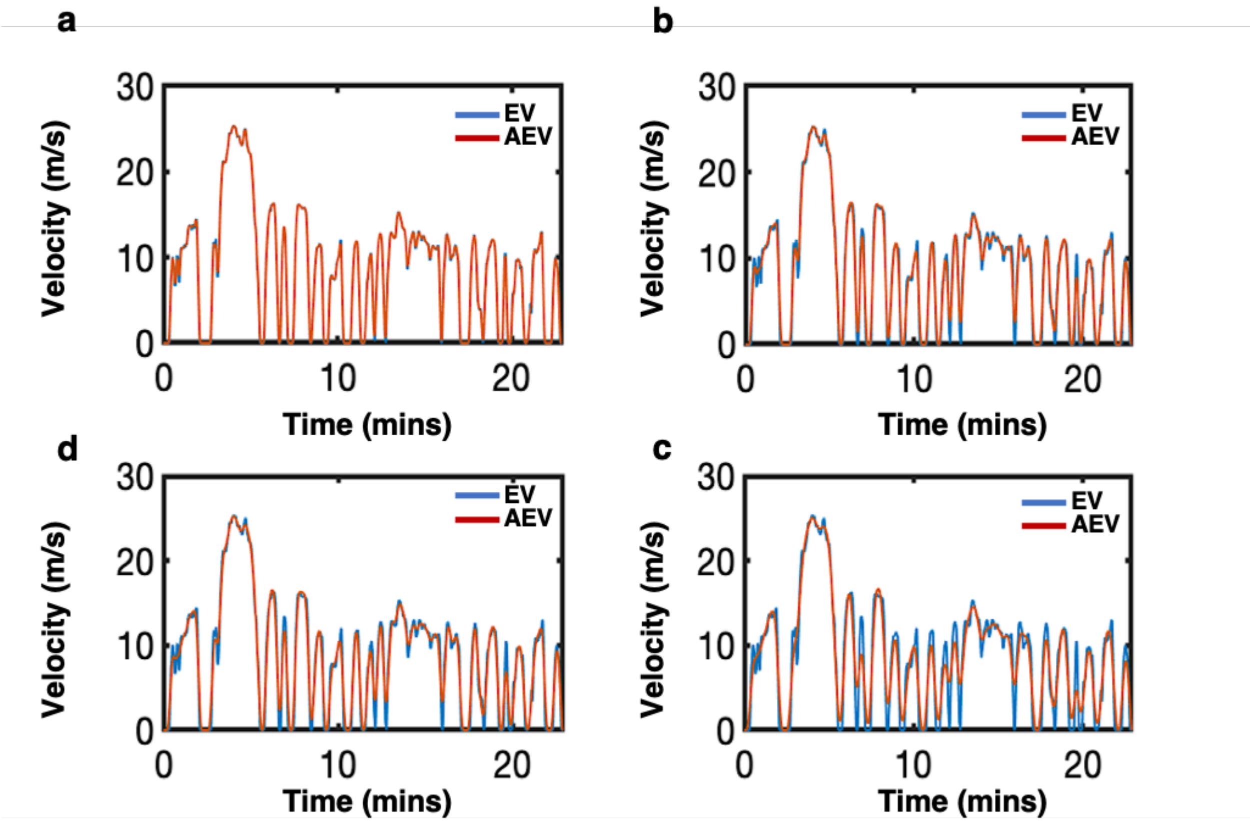


**Figure S3:** City cycle: Clockwise from Left to Right **a**, AEV vs EV drive cycle for 5% energy savings, **b**, AEV vs V drive cycle for 10% energy savings. **c**, AEV vs EV drive cycle for 20% energy savings. **d**, AEV vs EV drive cycle for 25% energy savings.

We see in Figures b, c, and d that there are several moments with the vehicle is stopped in the original velocity profile (v=0), but has non-zero velocity in the smoothed profile. In the 25% energy saving case, the difference is perhaps untenable: the smoothed velocity is 10m/s (22mph or 36kmph) when the vehicle is stopped in the original velocity profile. This illustrate the limitations of our approach to drive cycle smoothing and perhaps the difficulty of achieving big

savings through drive cycle smoothing in an urban context.

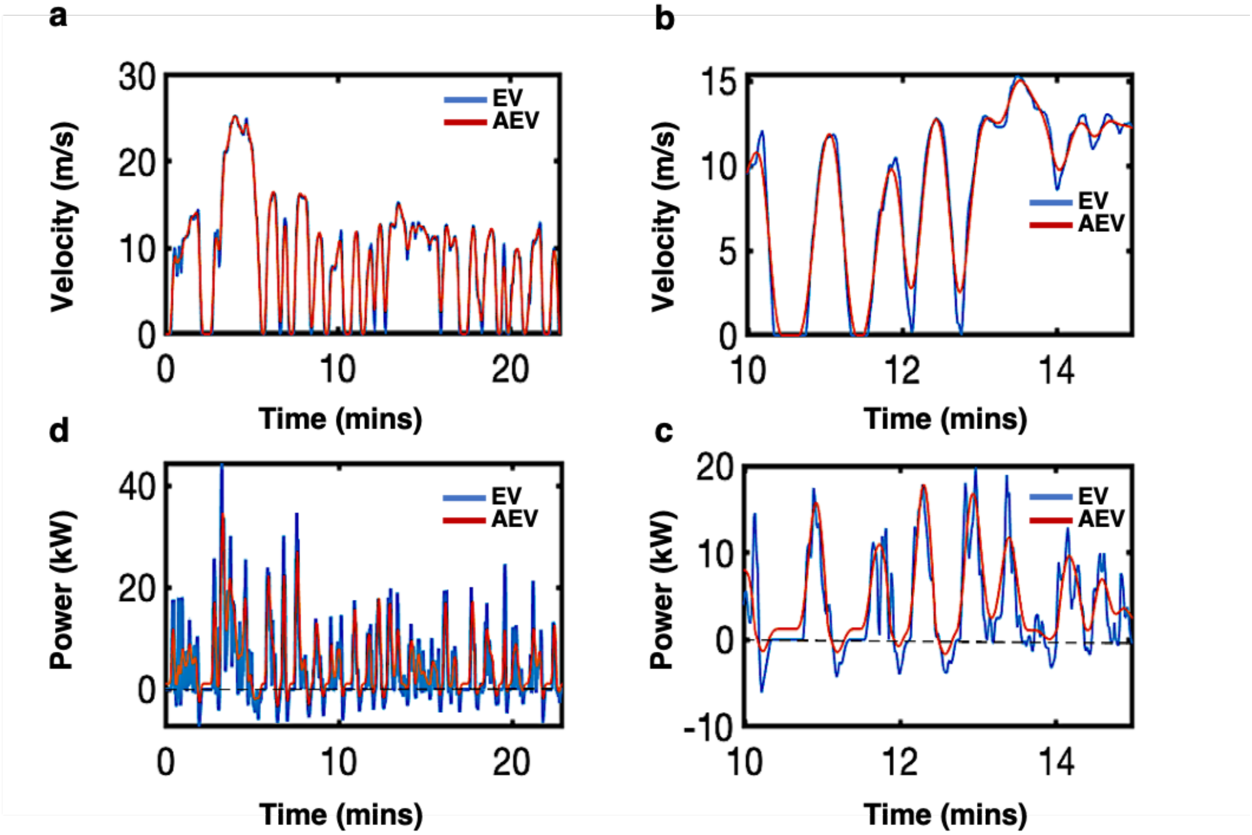


**Figure S4:** Clockwise from Left to Right: **a**, The city drive cycle for an EV vs an AEV with 10% energy savings. **b**, A zoomed in look at the smoothing of the drive cycle between minutes 10 to 15 which shows the effect of smoothing on braking and acceleration **c**, The corresponding power profiles for a Tesla Model 3 EV and AEV, assuming a 1000 W compute load, 150 W sensor load, 25% increase in drag from LiDAR and 10% energy savings from smoother driving. **d**, A zoomed in look at the power profile between minutes 10 to 15.

This plot provides a closer look at the smoothing of the city drive cycle; it is the counterpart to Figure 1 in the main paper which shows the same effect but for the composite drive profile. In both cases energy savings are mainly achieved through gentler braking and smoother acceleration.

## 4 Box Plot results for different EV models (city profile)

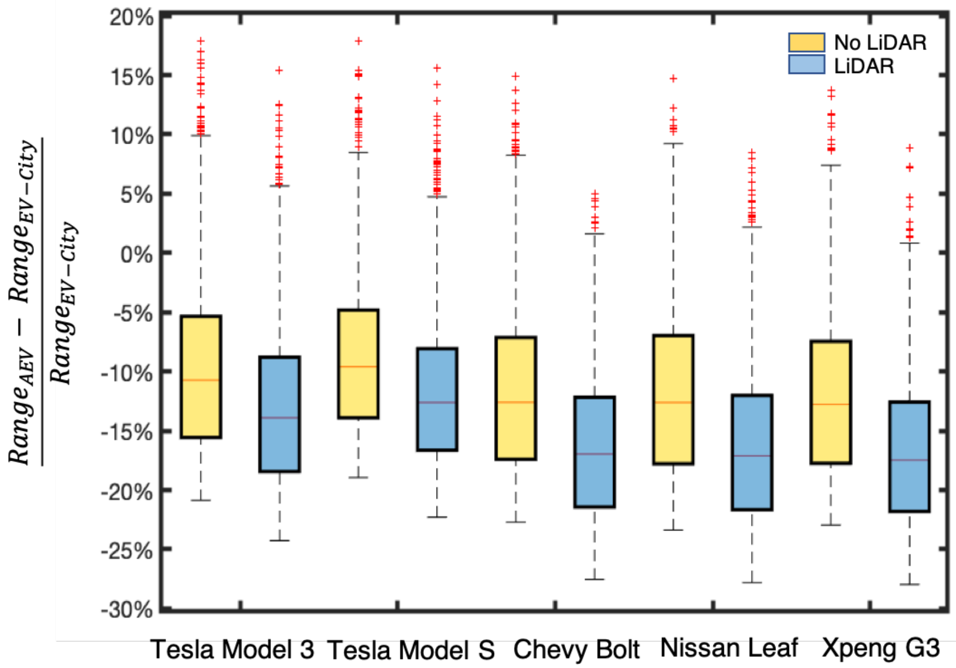


**Figure S5:** Box plot shows the results of the Monte Carlo analysis for different EV models for the city drive profile and for autonomous solutions with and without LiDAR. We estimate the baseline EV city ranges by running our physics model for the different EVs with the city driving profile. This estimated baseline range is then compared to the Monte Carlo results from simulating the case of corresponding AEVs with and without LiDAR.

This plot is the counterpart to Figure 3 in the main paper which shows the results for the city-highway composite profile. Comparing the two we can see that going from EVs to AEVs while driving a city velocity profile results in a greater percentage reduction in range for all the EVs we analyze, regardless of whether we assume increased drag from the presence of LiDAR. This is because the average velocity in city profiles is low, resulting in a small penalty from increased

drag (which increases as the cube of the velocity). The energy penalty associated with automation is therefore dominated by the increase in computational loads, which we assume are constant over time and velocity. Due to lower city velocities, the vehicle runs for a longer duration than it does in the city-highway composite cycle, before its range is exhausted. As such, the total energy use for computation is higher for the city drive profile than it is for other drive profiles with lower average velocities. We can also see that the difference between the case with LiDAR and without is smaller for the city profile compared to the composite profile due to slower speeds in the city which result in a lower impact from additional drag.

## 5 Sensitivity analysis of results

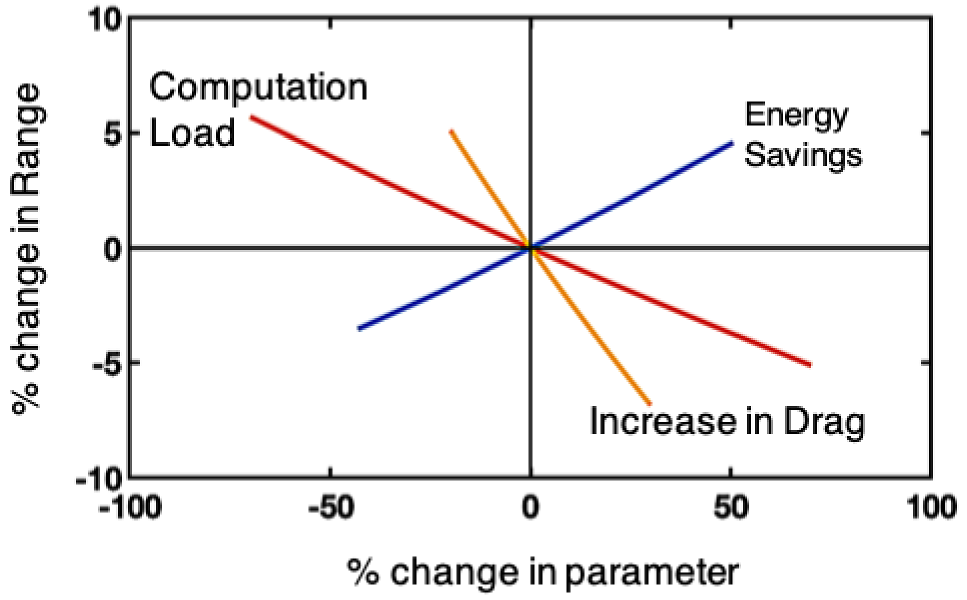


**Figure S6:** Sensitivity plot of changes in range for the composite drive profile which shows that estimates of the increase in drag from LiDAR is the most sensitive input parameter in our model, followed by compute load and energy savings of smoother driving.

Even doubling the computing load results in less than a 10% decrease in range whereas if LiDAR increases the drag experienced by a vehicle by 50%, it will lead to more than a 10% loss in range. Changes in sensor load has minimal impact on range and was therefore not plotted on the figure.

## 6 Battery degradation results

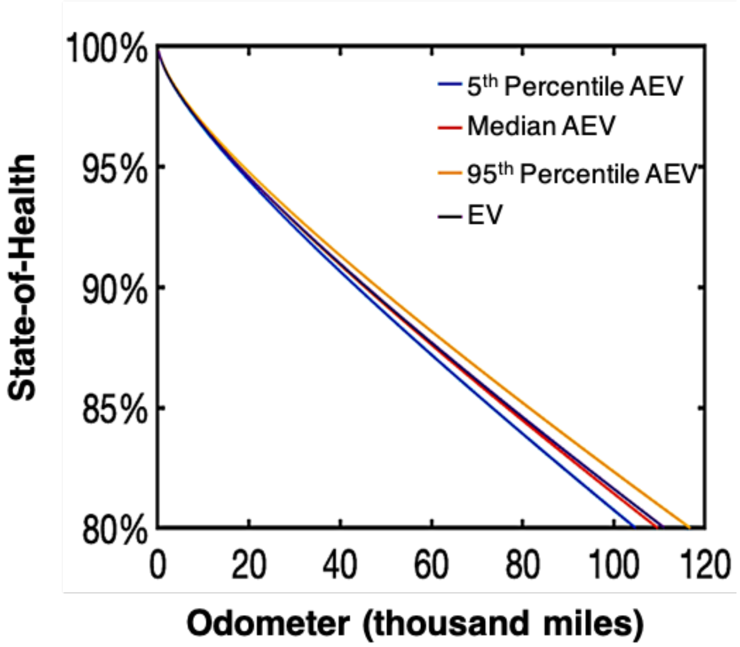


**Figure S7:** Battery degradation of the AEV Model 3 without LiDAR and the EV Model 3 for the composite drive cycle and a daily drive schedule of 50 miles. The median AEV without LiDAR lasts for approximately 110,000 miles and the 5th percentile AEV lasts for approximately 105,000 miles. The median loss in battery longevity compared to the EV is 1,300 miles or a month of driving. The 5th percentile case leads to a loss of 6,000 miles or four months of driving compared to the EV.

The reduction in battery longevity above can be compared to Figure 4 in the main paper which shows the results for the composite cycle with LiDAR compared to the EV. Comparing the two we can see that AEVs without LiDAR have slower degradation of battery longevity compared to AEVs with LiDAR, with the elimination of LiDAR resulting in an additional 4,000 miles of battery longevity.

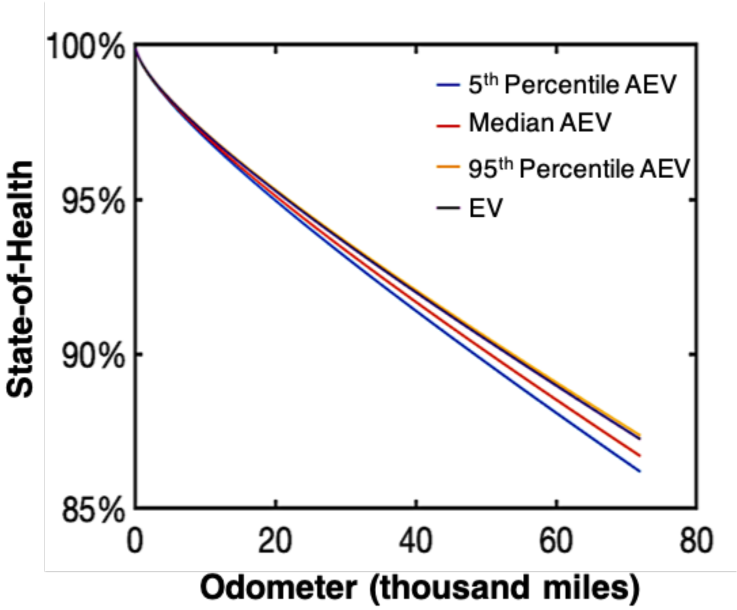


**Figure S8:** Battery degradation of the AEV Model 3 with LiDAR and the EV Model 3 for the city drive cycle and a daily drive schedule of 30 miles. We model 2,400 cycles similar to the composite profile shown previously. State of health does not drop to 80% in this case, reflecting the fact that the city drive profile and the lower daily drive schedule of 30 miles instead of 50 result in slower battery degradation. At 90% state of health the EV has completed 2,500 miles more than the median AEV.

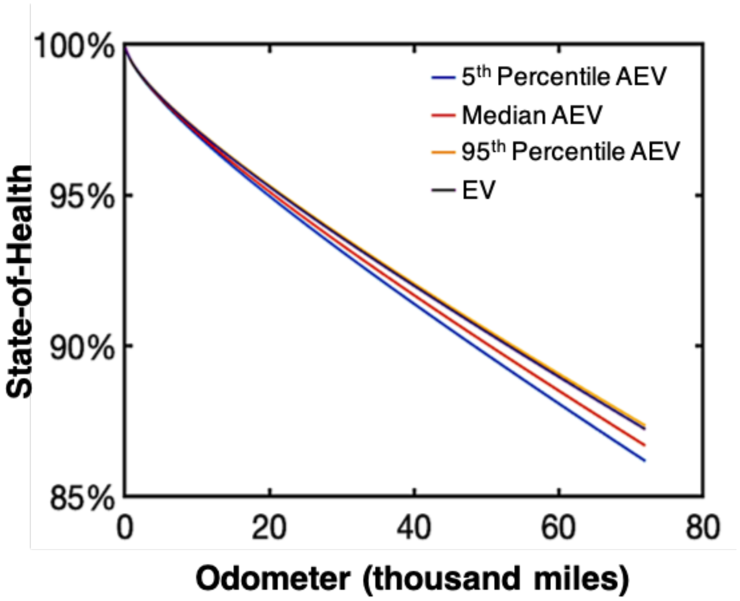


**Figure S9:** Battery degradation of the AEV Model 3 without LiDAR and the EV Model 3 for the city drive cycle and a daily drive schedule of 30 miles. Again, state of health does not drop to 80% even after 2,400 cycles. At 90% state of health the EV has completed only 500 miles more than the median AEV. Eliminating LiDAR therefore also increases battery longevity in the city profile.

## 7 Costs of automation: Willingness to pay

**Table S1:** Willingness to pay for range likely does not exceed $100 per mile based on the prices of current EVs

<table>
<tr><th>Model</th><th>Range (miles)</th><th>Price ($)</th><th>WTP / mi.</th><th>WTP 10% of range</th></tr>
<tr><td>BMW i3</td><td>153</td><td>44450</td><td rowspan="2">82</td><td rowspan="2">1253</td></tr>
<tr><td>BMW i3 with range extender</td><td>200</td><td>48300</td></tr>
<tr><td>BMW i3s</td><td>153</td><td>47560</td><td rowspan="2">84</td><td rowspan="2">1283</td></tr>
<tr><td>BMW i3s with range extender</td><td>200</td><td>51500</td></tr>
<tr><td>Nissan Leaf</td><td>151</td><td>30795</td><td rowspan="2">73</td><td rowspan="2">1107</td></tr>
<tr><td>Nissan Leaf Plus</td><td>226</td><td>36295</td></tr>
</table>

We estimate how much customers are willing to pay upfront for an additional mile of range by comparing identical or near-identical vehicles that differ merely in range. Note that this is also an estimate of what customers are willing to accept in return for a mile of lost range: effectively, buyers of a BMW i3 without range extender, accepts $3,850 in exchange for the additional 47 miles of range that a range extender would buy them. This leads us to conclude that consumers may not be willing to pay more than $100 upfront per mile of range, which is in line with surveys that show how much customers value range. As such, we would expect then to value the approximately 30-mile loss in range at no more than $3000.
